# Supplementary material for: Direct observation and evolution of electronic coupling between organic semiconductors
Source: arXiv:2008.04641 ancillary file (2020-11-17)
Supplement: Supplementary file 1 [file SupplementaryInformation.pdf]

## Supplementary Information: Direct observation and evolution of electronic coupling between organic semiconductors

Sameer Vajjala Kesava, Moritz K. Riede

Department of Physics, University of Oxford, OX1 3PU, Oxford, UK

### S1. Derivation of $\delta\rho$

Consider a film with in-plane and out-of-plane refractive index  $N_{1xy}$ ,  $N_{1z}$  respectively being deposited on a substrate with refractive index  $N_2$  under vacuum  $N_0$  and being monitored in-situ using a spectroscopic ellipsometer at an angle of incidence  $\theta_0$  ( $65^\circ$  in our setup) as shown in Figure S1. The refractive indices are functions of wavelength  $\lambda$ .

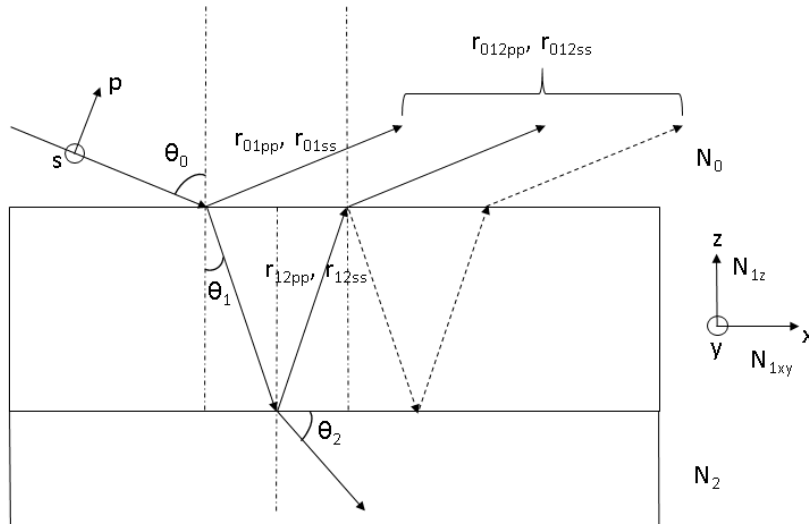

**Figure S1.** Ratio of reflection coefficients  $r_{012pp}$  and  $r_{012ss}$  measured in standard SE.  $N_0$  is vacuum refractive index,  $N_{1xy}$  and  $N_{1z}$  are in-plane and out-of-plane refractive indices of the thin film being deposited on substrate  $N_2$ .

The ellipsometric ratio  $\rho$  measured at any time point  $t$  (thickness  $d$ ) is given by

$$\rho = \frac{r_{012pp}}{r_{012ss}} \quad \text{Equation S1.1}$$

$r_{012pp}$  and  $r_{012ss}$  are the total reflection coefficients of the  $p$  and  $s$  polarizations of the electric field of the probe light, and given by the following equations. For  $p$ -polarization,

$$r_{012pp} = \frac{r_{01pp} + r_{12pp} e^{-j2\beta_p}}{1 + r_{01pp} r_{12pp} e^{-j2\beta_p}} ; \quad r_{012ss} = \frac{r_{01ss} + r_{12ss} e^{-j2\beta_s}}{1 + r_{01ss} r_{12ss} e^{-j2\beta_s}} \quad \text{Equations S1.2(a), (b)}$$

$$r_{01pp} = \frac{N_{1xy} N_{1z} \cos \theta_0 - N_0 (N_{1z}^2 - N_0^2 \sin^2 \theta_0)^{1/2}}{N_{1xy} N_{1z} \cos \theta_0 + N_0 (N_{1z}^2 - N_0^2 \sin^2 \theta_0)^{1/2}} \quad \text{Equation S1.3(a)}$$

$$r_{12pp} = \frac{N_2 (N_{1z}^2 - N_2^2 \sin^2 \theta_2)^{1/2} - N_{1xy} N_{1z} \cos \theta_2}{N_2 (N_{1z}^2 - N_2^2 \sin^2 \theta_2)^{1/2} + N_{1xy} N_{1z} \cos \theta_2} \quad \text{Equation S1.3(b)}$$

$$\beta_p = \frac{2\pi d}{\lambda} \frac{N_{1xy}}{N_{1z}} (N_{1z}^2 - N_0^2 \sin^2 \theta_0)^{1/2} \quad \text{Equation S1.3(c)}$$

Similarly, for  $s$ -polarization,

$$r_{01ss} = \frac{N_0 \cos \theta_0 - (N_{1xy}^2 - N_0^2 \sin^2 \theta_0)^{1/2}}{N_0 \cos \theta_0 + (N_{1xy}^2 - N_0^2 \sin^2 \theta_0)^{1/2}} \quad \text{Equation S1.4(a)}$$

$$r_{12ss} = \frac{(N_{1xy}^2 - N_2^2 \sin^2 \theta_2)^{1/2} - N_2 \cos \theta_2}{(N_{1xy}^2 - N_2^2 \sin^2 \theta_2)^{1/2} + N_2 \cos \theta_2} \quad \text{Equation S1.4(b)}$$

$$\beta_s = \frac{2\pi d}{\lambda} (N_{1xy}^2 - N_0^2 \sin^2 \theta_0)^{1/2} \quad \text{Equation S1.4(c)}$$

In short,  $r_{012pp}$  and  $r_{012ss}$  are functions of  $N_{1xy}$ ,  $N_{1z}$ ,  $d$ . For more details on the derivations of these equations, please refer to references 1 and 2<sup>1,2</sup>.

$$r_{012pp} = F(N_{1xy}, N_{1z}, d); \quad r_{012ss} = G(N_{1xy}, d) \quad \text{Equation S1.5}$$

The first derivative of  $\rho$  with respect to time  $t$  (or thickness  $d$ ) is given by

$$\frac{\delta \rho}{\delta t} = \frac{1}{r_{012ss}} \frac{\delta r_{012pp}}{\delta t} - \frac{r_{012pp}}{r_{012ss}^2} \frac{\delta r_{012ss}}{\delta t} \quad \text{Equation S1.6}$$

SE is a surface-sensitive technique, and thus is highly sensitive to changes in the properties of the film along the  $z$  direction, i.e.  $\delta \rho$  is sensitive to  $\delta d$  and  $\delta N_{1z}$ . Secondly, for the deposition

of pristine films, the in-plane environment of a molecule varies little or zero with thickness implying that  $\delta N_{1xy}$  can be reasonably approximated to 0. Consequently, the functions  $r_{012pp}$  and  $r_{012ss}$  can be approximated as

$$r_{012pp} \sim F(N_{1z}(d), N_{1xy}, d); r_{012ss} \sim G(d, N_{1xy}) \quad \text{Equation S1.7}$$

where  $N_{1z}$  is written as a function of  $d$  and  $N_{1xy}$  is assumed to be constant. Thus, the first derivatives of  $r_{012pp}$  and  $r_{012ss}$  with respect to  $t$  are

$$\frac{\delta r_{012pp}}{\delta t} \sim F' \left( N_{1z}(d), d, \frac{\delta N_{1z}(d)}{\delta t}, \frac{\delta d}{\delta t}, N_{1xy} \right); \quad \frac{\delta r_{012ss}}{\delta t} \sim G' \left( d, \frac{\delta d}{\delta t}, N_{1xy} \right) \quad \text{Equation S1.8}$$

With  $\delta d/\delta t$  being the rate of deposition, from equations S1.6 and S1.8, we can see that  $\delta \rho/\delta t$  is a function of the rate of change in the optical properties of the growing thin film along the thickness/ $z$  direction, i.e.  $\delta N_{1z}/\delta t$ . If  $N_{1z}$  does not change with deposition, implies  $\delta N_{1z}/\delta t = 0$ , and consequently  $\delta \rho/\delta t$  will be approximately constant for all thicknesses (approximate because  $d$  is increasing but only plays the role of a scaling factor through  $\beta_s$  and  $\beta_p$ ).

When implementing the equations in the main text, care needs be taken when calculating the differential  $\delta \Delta$ . Since  $\Delta$  is cyclic, i.e. varies from  $0^\circ$ - $360^\circ$  and after  $360^\circ$  the value starts from  $0^\circ$  again, it needs to be corrected for the same wavelength (or energy) during the calculation of  $\delta \Delta$ . The following set of instructions must be used.

For any two consecutive time points,  $t$  and  $t+1$ ,

$$\text{if } \Delta_{t+1} - \Delta_t > 180^\circ, \text{ then } \Delta_{t+1} = \Delta_{t+1} - 360^\circ$$

$$\text{else, if } \Delta_{t+1} - \Delta_t < -180^\circ, \text{ then } \Delta_{t+1} = \Delta_{t+1} + 360^\circ$$

This modification of  $\Delta$  does not change the  $\rho$  value (both real and imaginary).

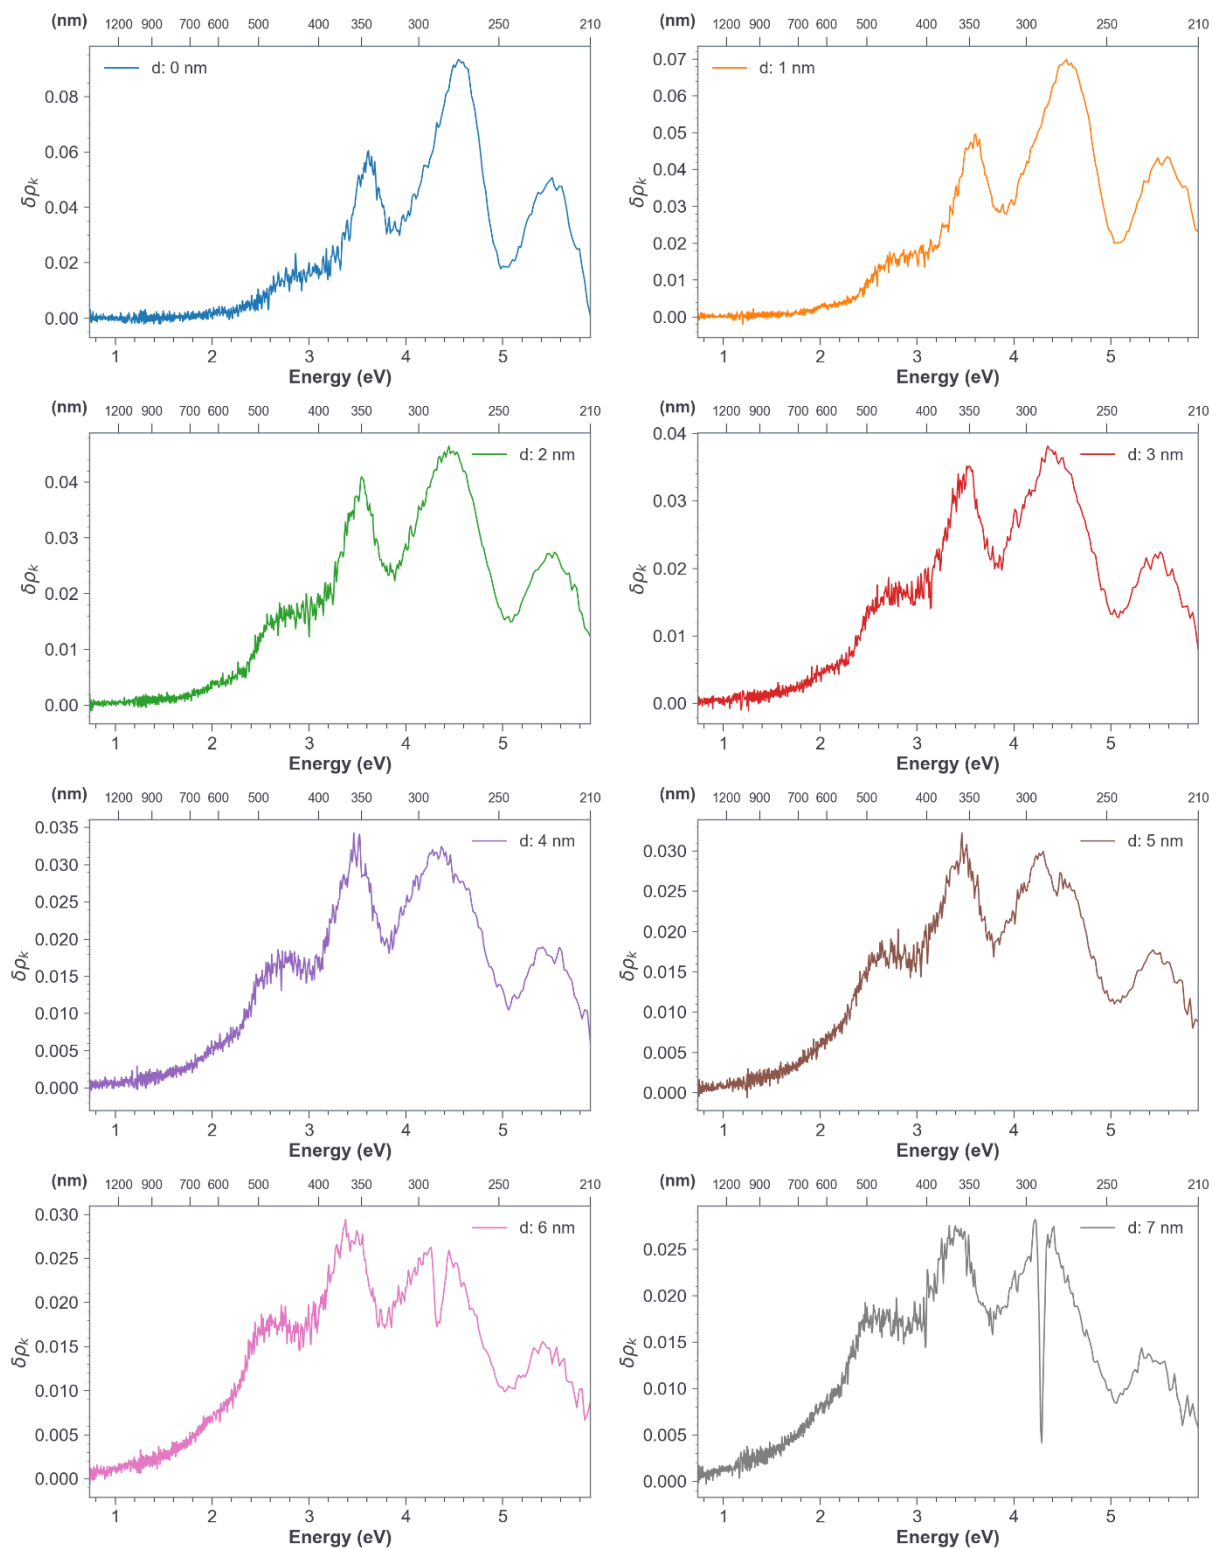

**Figure S2-I.** DART results (only  $\delta\rho_k$ ) of C60 deposited on SiO<sub>2</sub> (from Figure 1) displayed individually per nanometer until 7 nm for clear visualization. Continued next page.

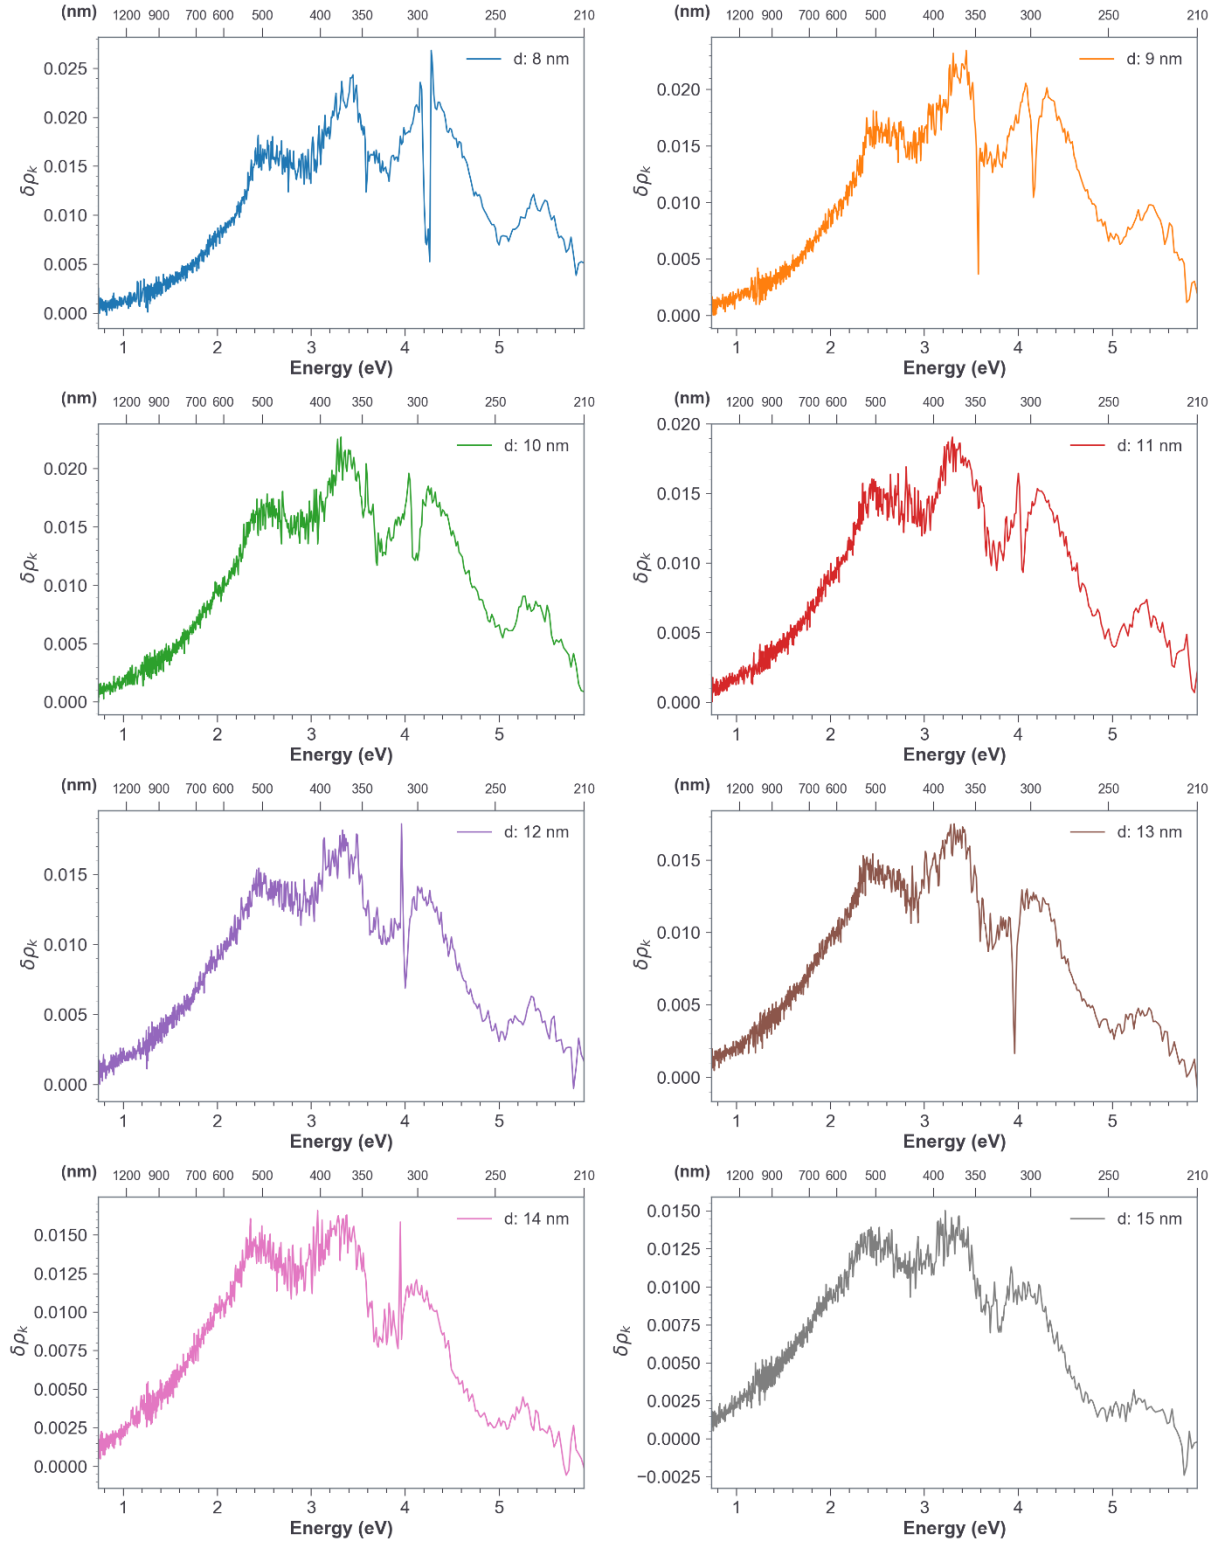

**Figure S2-II.** Continued from S2-I. DART results (only  $\delta\rho_k$ ) of C60 deposited on  $\text{SiO}_2$  substrate from (Figure 1) displayed individually per nanometer from 8 nm until 15 nm for clear visualization.



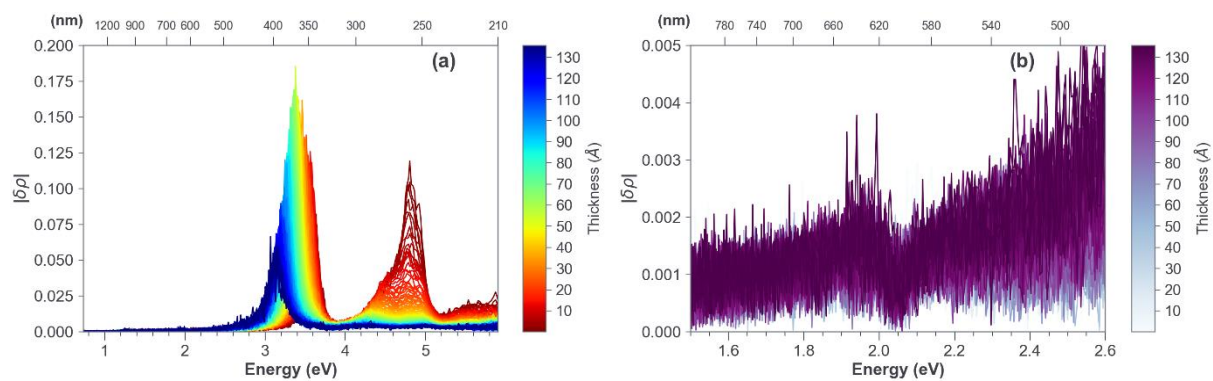

**Figure S4.** (a) DART analysis of C60 deposited onto the SubPc film (of Figure 4), calculated for a differential change of  $\delta d = 1 \text{ \AA}$ . (b) Magnified view of (a) showing the O1 transition signal (noisy here unlike in Figure 4(b).2) around 2.04 eV of the buried SubPc film.

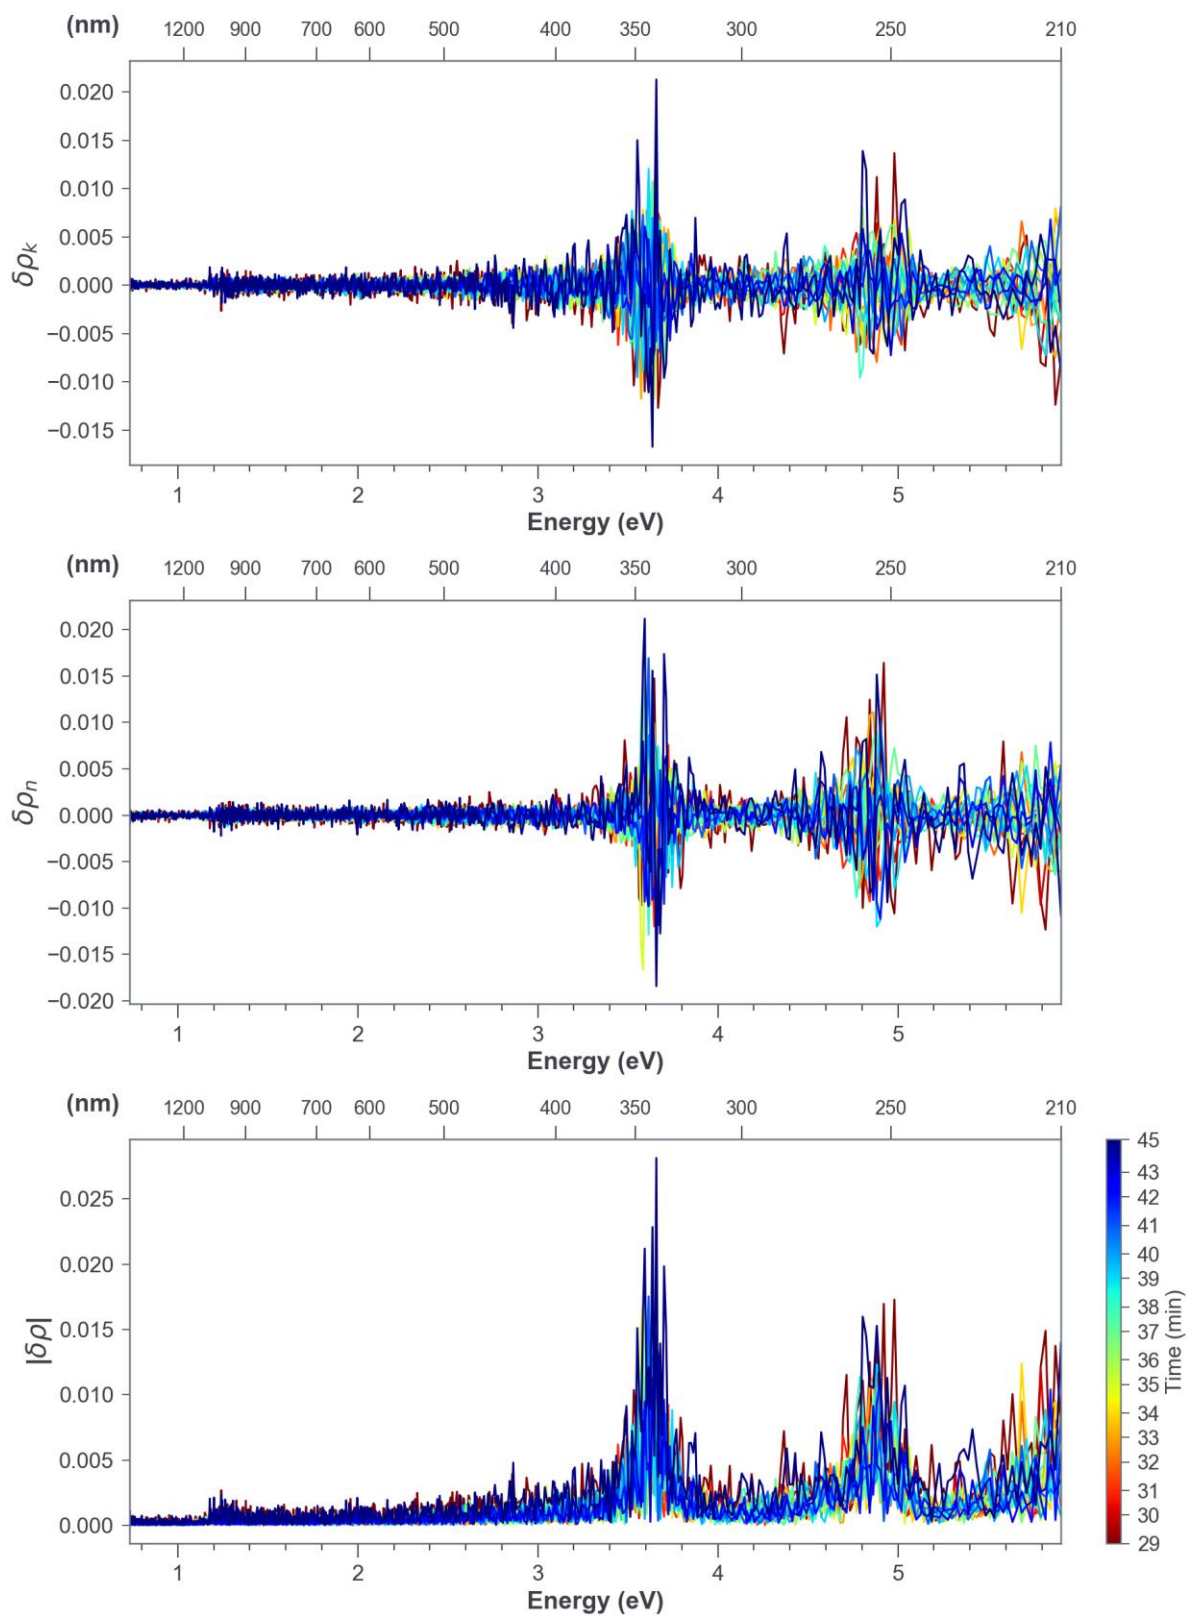

**Figure S5.** DART analysis of the iSE data obtained during the downtime between the end of SubPc deposition and start of C60 deposition corresponding to the films of Figure 4.  $\delta\rho$  was calculated for a differential change of  $\delta t = 1$  min.

## S2. Standard spectroscopic ellipsometry data analysis (SSE)

### Derivation of thickness:

For obtaining thicknesses from SE, a Cauchy model<sup>1</sup> was fit to a bulk or completed film of the pristine organic semiconductor, e.g. C60 film on SiO<sub>2</sub> at 26 nm thickness, in the transparent region ( $k=0$ ) for the refractive index  $n(\lambda)$ . This value was then used to obtain the thickness and roughness of the film at earlier time points including up to 1 nm. Low roughness (maximum of 1-2 nm) was obtained at all time points during growth indicating that all the films were deposited approximately smoothly.

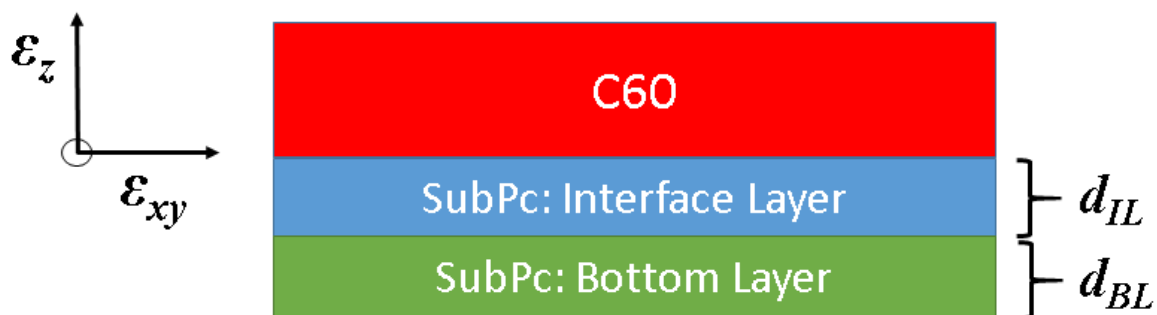

**Figure S6.** Schematic of the method used to derive the out-of-plane dielectric constants ( $\epsilon_z$ ) of the interface layer of SubPc using standard spectroscopic ellipsometry data analysis method (SSE). The buried layer (SubPc here as an example) onto which C60 is deposited is divided into an interface layer with C60 of thickness  $d_{IL}$  and a bottom layer  $d_{BL}$ .  $\epsilon_{xy}$  is the in-plane dielectric constant of a layer.

### Derivation of dielectric constants:

Strong electronic coupling along the vertical direction between C60 and phthalocyanines implies variation in  $N_z$  with thickness  $d$  ( $\delta N_z \neq 0$ ). Thus, to ensure  $\epsilon_z$  ( $\equiv N_z$ ) of C60 is obtained correctly for a bilayer system, isotropic dielectric constants  $\epsilon$  of C60 film deposited on SiO<sub>2</sub>

(optically smooth quartz substrate) were obtained by fitting to the iSE data at 13 nm C60 thickness (values were similar to that at 26 nm C60 thickness). These values were then used as the in-plane dielectric constants  $\epsilon_{xy}$  of C60 deposited on phthalocyanines since the in-plane environment of a bulk or completed C60 film is determined by the C60 molecules, and thus can be taken as unchanged when deposited on an interacting substrate such as phthalocyanines. Moreover, the millimeter size footprint of the probe light in xy direction also ensures that the average optical properties measured along the xy direction remains constant with homogenous deposition.

$\epsilon_{xy}$  of C60 was fixed as above, and for SubPc (both IL<sub>SubPc</sub> and BL<sub>SubPc</sub>)  $\epsilon_{xy}$  was set equal to the values obtained from model fitting to the data before C60 deposition (Figure S3 (e) and (f)) and assumed as unchanging upon C60 deposition since the xy environment remains the same (to a first or even higher order approximation). For IL<sub>SubPc</sub>, the  $\epsilon_z$  Gaussian oscillators from Figure S3 (e) and (f) were used as the starting parameters, and BL<sub>SubPc</sub>  $\epsilon_z$  was set the same values as before C60 deposition from Figure S3 (e) and (f). Then, obtaining  $\epsilon_z$  of C60 and IL<sub>SubPc</sub> of the bilayer system shown in Figure S6 (and the inset of Figure 5(b)) follows the usual SSE approach of fitting the dielectric function model using the Gaussian oscillators leading to observation of resonances. One needs to be careful when fitting for  $\epsilon_z$  in energy ranges which correspond to overlapping absorptions between the top and bottom/underlying layers. In our case, C60  $\epsilon_z$  was fit for energy ranges 2.3-4.0 eV since including energies below 2.3 eV led to features in C60  $\epsilon_z$  around the  $\pi$ - $\pi^*$  transition energies which in reality correspond to SubPc (and SubNc), i.e. around 1.8-2.3 eV (1.6-2.3 eV for SubNc). Similarly, when fitting for  $\epsilon_z$  of the IL<sub>SubPc</sub> interface layer (same for SubNc), it was carried out for energy ranges less than 2.3 eV only since including higher energies lead to absorption in the transparent region, i.e. around 3.0 eV which is not physical. This is because the fitting algorithm subsumes any absorption in the top C60 layer into the underlying  $d_{IL}$  layer and vice versa in order to reduce the mean

squared error (MSE) when fitting one layer at a time. Unfortunately,  $\epsilon_z$  of C60 and  $IL_{SubPc}$  cannot be fit together since the number of parameters to be determined (4: real and imaginary parts of both the layers) are more than the number of data points (2:  $\psi$  and  $\Delta$ ) which leads to overfitting. Attempting this, anyways, led to high correlation between the fit parameters of the Gaussian oscillators of C60  $\epsilon_z$  and SubPc  $\epsilon_z$ , and inconsistent results were obtained with different iterations. However, using the method defined above, i.e. fixing  $\epsilon_{xy}$  obtained from C60 on glass, led to highly consistent results of  $IL_{SubPc}$   $\epsilon_z$  and C60  $\epsilon_z$  (along with the trend observed in the DART results with increasing thickness) for all the different films as shown in Figures S7 and S8 respectively along with good fit statistics of the parameters (Table S1). But this might not work if the molecule on the top layer is not isotropic, e.g. tetracene, SubPc and SubNc, since in this case  $\epsilon_{xy}$  cannot be known unless one can determine from, for example, in-situ X-ray scattering measurements the orientation at each time point during the deposition.

Variation of  $\epsilon_z$  of  $IL_{SubPc}$  layers with thickness  $d_{ILSubPc}$  deposited on  $SiO_2$ , MoOx and PrT is shown in Figure S7 (also for SubNc). Since in SSE analysis, a film is usually analysed starting with the assumption that it has uniform properties along its thickness, any absorption feature arising at a particular point along the thickness in the film – mostly commonly the interfaces – is averaged out across the whole film by the fitting algorithm since its purpose is to reduce MSE for the uniform model. This means that instead of yielding a strong oscillator (absorption coefficient) at that point, for example, near an interface, the analysis results in a weak oscillator spread across the film to be able to account for the average absorption of the complete layer; even with additional optical data from ex-situ measurements it is extraordinarily challenging to isolate the features because of the way the SSE analysis works<sup>1</sup>. In light of this aspect of SSE fitting, if the 2.04 eV  $|\delta\rho|$  feature at the interface with C60 in Figure 4(b).2 (also Figures S6(b).2, S9(b).2 and S10(b).2) does correspond to the resonance oscillator (transition) O1 in the  $IL_{SubPc}$  layer, then increasing  $d_{ILSubPc}$  should result in the decrease in the O1's  $\epsilon_{2z}$  value

because of the averaging across the thickness by the algorithm to reduce the MSE. This trend in  $\epsilon_{2z}$  is visible in Figure S7(a), which shows that, firstly, the O1 transition strength increases compared to its value before C60 deposition when the whole bulk film itself is analysed during fitting, i.e.  $d_{ILSubPc} = \text{full layer thickness of 16 nm}$  ( $d_{BLSubPc} = 0$ ). Thereafter, it increases as  $d_{ILSubPc}$  decreases (while adjusting  $d_{BLSubPc}$  to keep the total thickness constant) with resonance thickness  $d_{ILSubPc}^{Res} = 1 \text{ nm}$  for SubPc on SiO<sub>2</sub>, (0.8 nm for SubPc on MoOx and 1.2 nm for SubPc on PrT), confirming that the 2.04 eV  $|\delta\rho|$  feature is the O1 transition. The Gaussian fit statistics of the O1 transition are shown in Table S1 indicating high confidence in the fitting.

Variation of  $\epsilon_z$  of the top C60 layers with its thickness deposited on SubPc<sub>SiO2</sub>, SubPc<sub>MoOx</sub> and SubPc<sub>PrT</sub> is shown in Figure S8 (also for SubNc).  $d_{ILSubPc}$  was set to the resonance thickness, i.e.  $d_{ILSubPc}^{Res}$ , in this analysis of the top C60 layer. The decrease in the resonance absorption of C60 with increase in its thickness is in conformity with the changes in the optical response  $|\delta\rho|$  of C60 with thickness shown in Figures 4(b).1, S9(b).1, S10(b).1 and 6(b).1, where the strength of the  $|\delta\rho|$  peaks increases until 4-5 nm and then starts decreasing. A difference to the DART results can be seen in the form of peak energies of the oscillators in C60  $\epsilon_{2z}$  which are centered at  $\sim 3 \text{ eV}$ . This, again, could be because a SSE analysis assuming homogeneous medium averages out any variation across the film thickness and relies on the accuracy of the model used for fitting.

### Issues with SSE:

The typical SSE approach starts by modelling the organic semiconductor films as composing of uniform, isotropic optical properties, i.e. same properties along x, y and z directions. Since the goal of the fitting algorithm is to reduce the mean-squared error and since  $\epsilon_{xy}$  (or  $N_{xy}$ ) is a function of both  $r_{pp}$  and  $r_{ss}$ , whereas  $\epsilon_z$  ( $N_z$ ) is only a function of  $r_{pp}$ , the fitting algorithm yields average  $\epsilon$  with significant weightage from  $\epsilon_{xy}$  for an isotropic model. Moreover, this average  $\epsilon$

is further averaged across the whole film rendering the approach all the more insensitive to variations in the properties due to wavefunction delocalization along the thickness and anomalous signatures due to electronic coupling at interfaces especially when the molecule is isotropic such as C60 even though the it's optical response is anisotropic as shown in our work. If the molecule itself is anisotropic such as SubPc and SubNc, the SSE approach can differentiate between  $\epsilon_{xy}$  and  $\epsilon_z$  but again, since the film is considered as composing uniform properties along the thickness direction, any interfacial couplings are undetected. This becomes more problematic in the case of two or more layers of semiconductors or other electronic materials, and worse in the case of overlapping absorptions, where strong electronic coupling occurs since, again, the typical approach assumes that the optical properties of the bottom layer has not changed after the deposition of the top layer. Since the goal of the fitting algorithm in the SSE approach is to minimize the overall MSE by fitting the parameters of the dielectric functions to the SE data, any changes in the bottom layer (after the deposition of the top layer) could show up in the dielectric constants of the top layer when fitting for its optical properties. These issues highlight the shortcomings of the SSE analysis approach of model fitting which can be overcome to a certain extent if complemented with additional real-time optical information such as differential reflectance spectroscopy<sup>4,5</sup>.

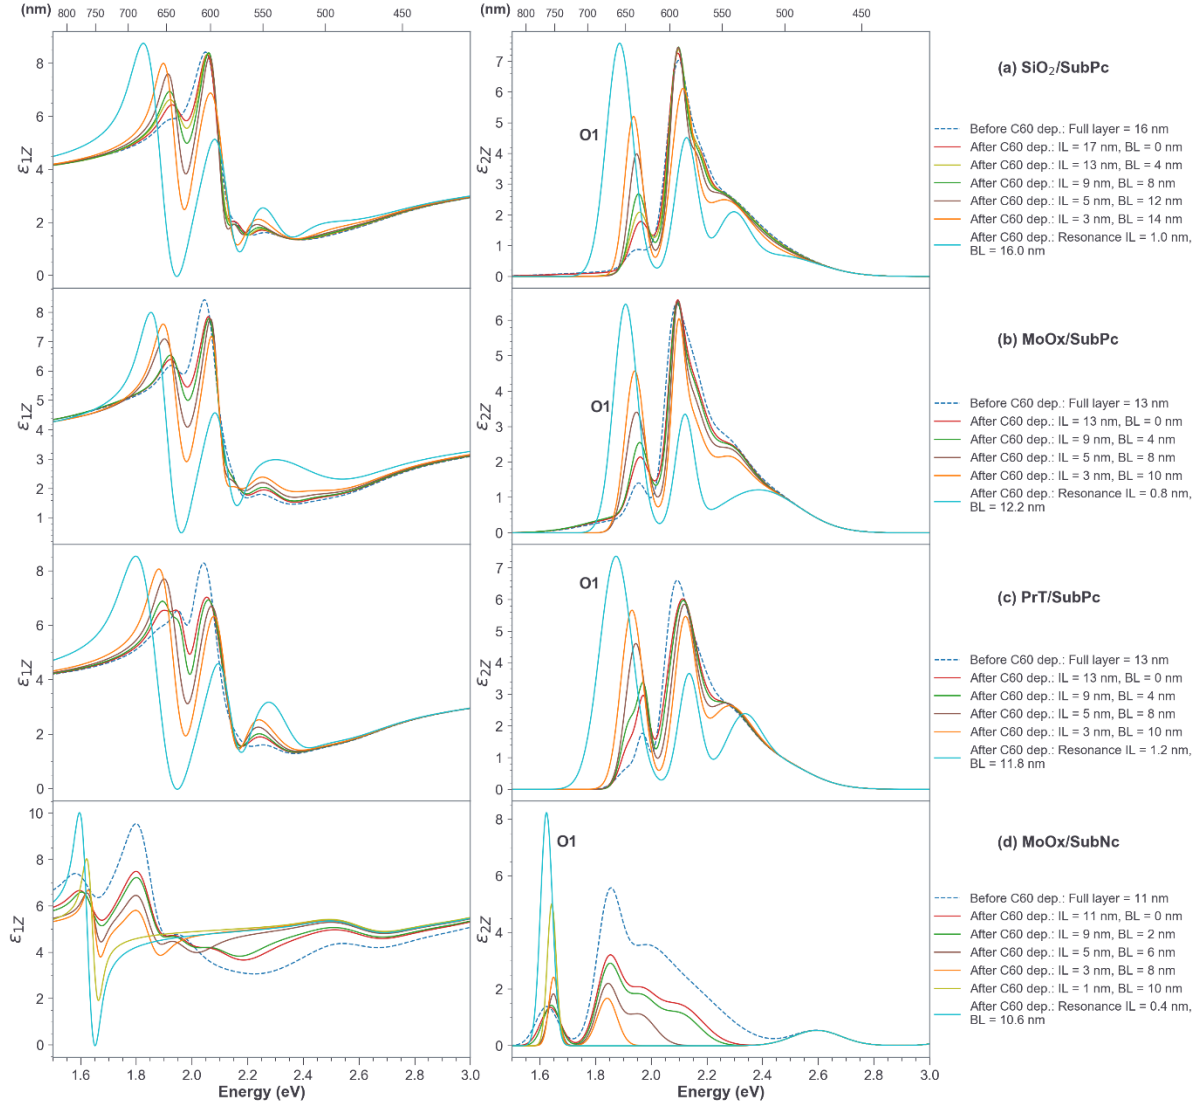

**Figure S7.** SSE analysis for  $\epsilon_z = \epsilon_{1z} + j \epsilon_{2z}$  (left:  $\epsilon_{1z}$ , right:  $\epsilon_{2z}$ ) of the interface SubPc layer ( $IL_{\text{SubPc}}$ ) as a function of its thickness after C60 (at 12 nm thickness) deposition for **(a)** SubPc on  $\text{SiO}_2$ , **(b)** SubPc on MoOx, **(c)** SubPc on PrT and **(d)** SubNc on MoOx.

**Table S1.** Estimates of the Gaussian fit parameters of the O1 transition of the phthalocyanines from fitting to iSE data. Parameters are Amplitude: A, Center Energy: E, Broadening: B.

| $d_{IL}$<br>(nm) | SiO <sub>2</sub> / <i>SubPc</i> /C60                                                                                          | SiO <sub>2</sub> /MoOx/<br><i>SubPc</i> /C60                                                                                  | SiO <sub>2</sub> /MoOx/<br>PrT/ <i>SubPc</i> /C60                                                                             | SiO <sub>2</sub> /MoOx/<br><i>SubNc</i> /C60                                                                                  |
|------------------|-------------------------------------------------------------------------------------------------------------------------------|-------------------------------------------------------------------------------------------------------------------------------|-------------------------------------------------------------------------------------------------------------------------------|-------------------------------------------------------------------------------------------------------------------------------|
| 16.0             | A = $1.317 \pm 0.207$<br>B = $0.074 \pm 0.013$<br>E = $1.958 \pm 0.006$                                                       |                                                                                                                               |                                                                                                                               |                                                                                                                               |
| 13.0             | A = $1.740 \pm 0.278$<br>B = $0.075 \pm 0.013$<br>E = $1.955 \pm 0.006$                                                       | A = $1.608 \pm 0.403$<br>B = $0.078 \pm 0.027$<br>E = $1.958 \pm 0.010$                                                       | A = $2.345 \pm 0.530$<br>B = $0.051 \pm 0.014$<br>E = $1.973 \pm 0.006$                                                       |                                                                                                                               |
| 11.0             |                                                                                                                               |                                                                                                                               |                                                                                                                               | A = $1.352 \pm 0.465$<br>B = $0.083 \pm 0.034$<br>E = $1.638 \pm 0.014$                                                       |
| 9.0              | A = $2.389 \pm 0.419$<br>B = $0.070 \pm 0.013$<br>E = $1.953 \pm 0.006$                                                       | A = $2.003 \pm 0.599$<br>B = $0.073 \pm 0.028$<br>E = $1.958 \pm 0.010$                                                       | A = $2.724 \pm 0.809$<br>B = $0.050 \pm 0.016$<br>E = $1.974 \pm 0.007$                                                       | A = $1.427 \pm 0.615$<br>B = $0.072 \pm 0.037$<br>E = $1.641 \pm 0.016$                                                       |
| 5.0              | A = $3.789 \pm 0.733$<br>B = $0.065 \pm 0.014$<br>E = $1.947 \pm 0.007$                                                       | A = $3.388 \pm 0.787$<br>B = $0.089 \pm 0.029$<br>E = $1.946 \pm 0.011$                                                       | A = $4.602 \pm 0.792$<br>B = $0.086 \pm 0.019$<br>E = $1.944 \pm 0.008$                                                       | A = $1.838 \pm 1.223$<br>B = $0.047 \pm 0.037$<br>E = $1.648 \pm 0.017$                                                       |
| 3.0              | A = $5.196 \pm 0.999$<br>B = $0.074 \pm 0.018$<br>E = $1.936 \pm 0.009$                                                       | A = $4.558 \pm 1.124$<br>B = $0.084 \pm 0.027$<br>E = $1.940 \pm 0.013$                                                       | A = $5.661 \pm 1.014$<br>B = $0.094 \pm 0.022$<br>E = $1.931 \pm 0.012$                                                       | A = $2.441 \pm 1.603$<br>B = $0.039 \pm 0.027$<br>E = $1.650 \pm 0.015$                                                       |
| 1.2              |                                                                                                                               |                                                                                                                               | <b>A = <math>7.369 \pm 1.244</math></b><br><b>B = <math>0.139 \pm 0.037</math></b><br><b>E = <math>1.874 \pm 0.029</math></b> |                                                                                                                               |
| 1.0              | <b>A = <math>7.588 \pm 1.361</math></b><br><b>B = <math>0.112 \pm 0.032</math></b><br><b>E = <math>1.886 \pm 0.024</math></b> |                                                                                                                               |                                                                                                                               | A = $5.013 \pm 3.213$<br>B = $0.038 \pm 0.021$<br>E = $1.642 \pm 0.015$                                                       |
| 0.8              |                                                                                                                               | <b>A = <math>7.163 \pm 1.684</math></b><br><b>B = <math>0.112 \pm 0.046</math></b><br><b>E = <math>1.892 \pm 0.036</math></b> |                                                                                                                               |                                                                                                                               |
| 0.4              |                                                                                                                               |                                                                                                                               |                                                                                                                               | <b>A = <math>8.241 \pm 3.514</math></b><br><b>B = <math>0.050 \pm 0.016</math></b><br><b>E = <math>1.624 \pm 0.014</math></b> |

Parameters in bold correspond to the O1 transition under resonance, i.e. when  $\varepsilon_{1z}$  becomes negative.

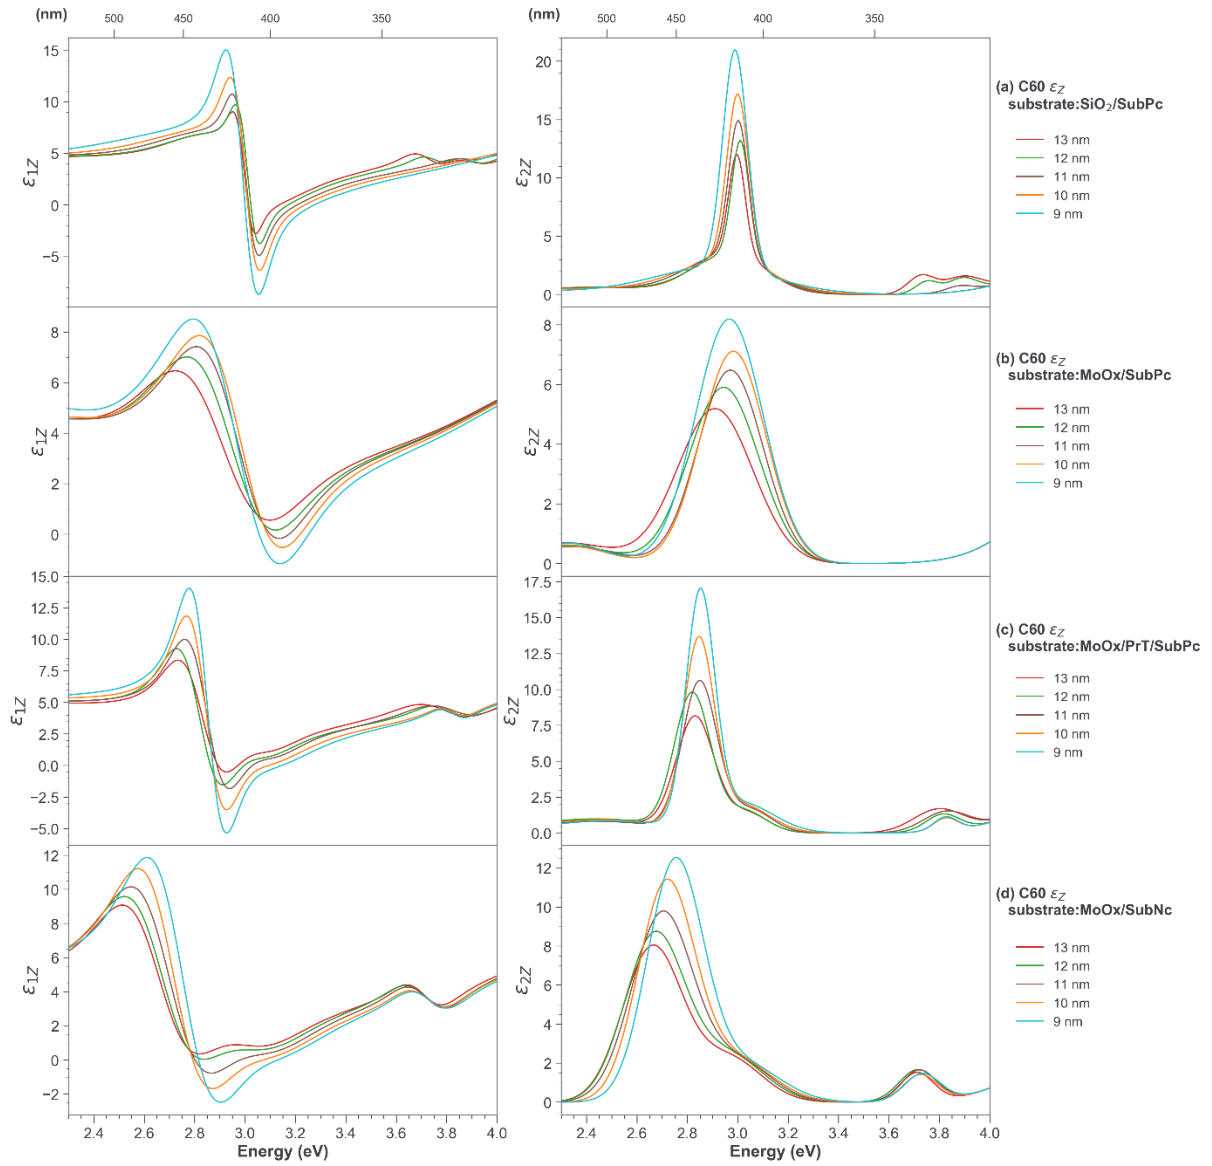

**Figure S8.** SSE analysis for resonance  $\epsilon_z$  (left:  $\epsilon_{1z}$ , right:  $\epsilon_{2z}$ ) of the top C60 layer as a function of its thickness deposited on **(a)** SiO<sub>2</sub>/SubPc, **(b)** MoOx/SubPc, **(c)** PrT/SubPc and **(d)** MoOx/SubNc.

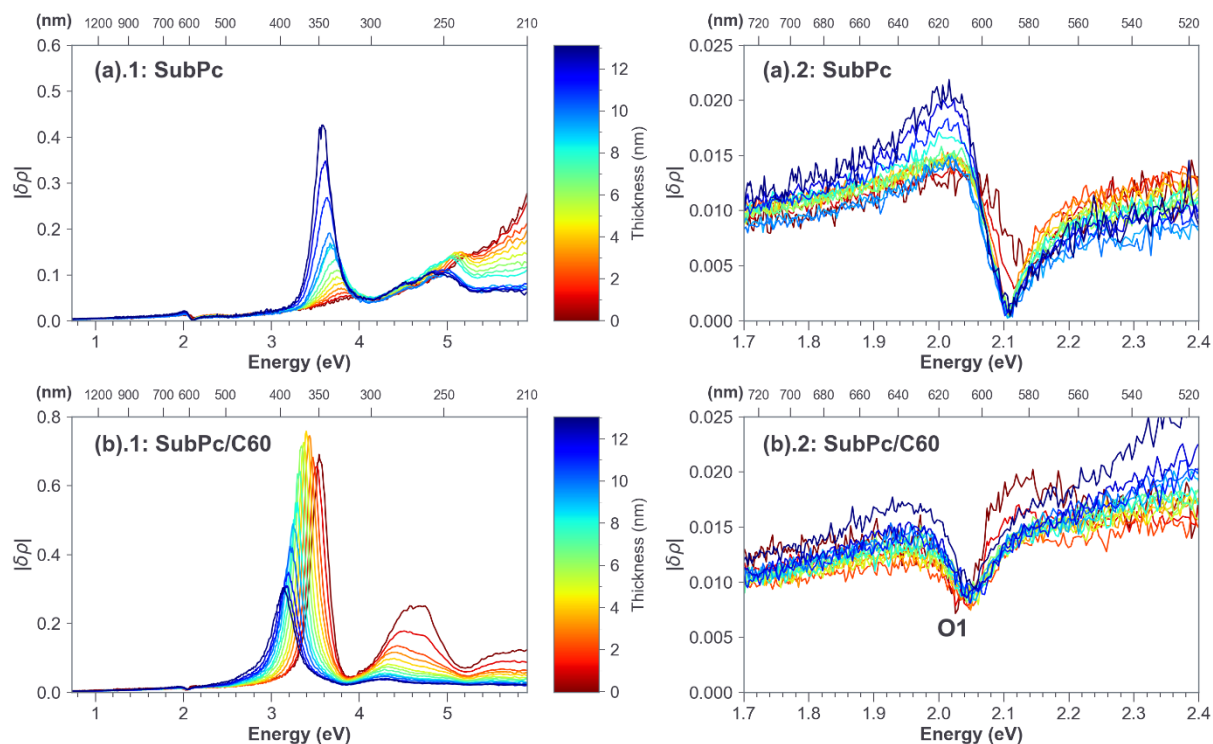

**Figure S9.** (a).1 DART analysis of a SubPc film deposited on Si/SiO<sub>2</sub>/MoOx<sup>6</sup>. (a).2 Magnified view of the same DART results in (a).1 showing the optical response corresponding to the  $\pi$ - $\pi^*$  transition<sup>3</sup> in SubPc for clear visualization. (b).1 DART analysis of C60 (analysed up to 13 nm thickness) deposited on the SubPc film in (a). (b).2 Magnified view of the data of (b).1 around 2.1 eV for clear visualization. The optical response corresponding to the excitations into SubPc excitonic states is indicated by the label O1. All calculations were carried out for a differential change of  $\delta d = 1$  nm.

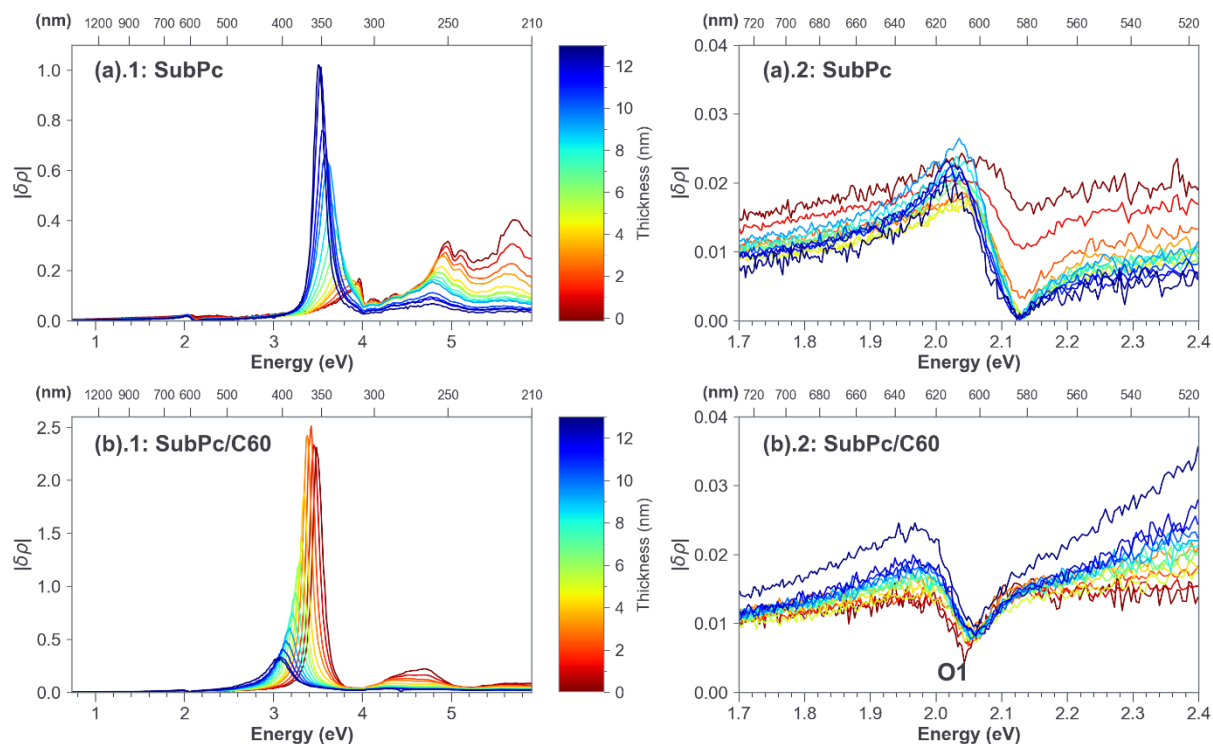

**Figure S10 (a).1** DART analysis of a SubPc film deposited on Si/SiO<sub>2</sub>/MoO<sub>x</sub>/PrT<sup>6</sup>. **(a).2** Magnified view of the same DART results in (a).1 showing the optical response corresponding to the  $\pi$ - $\pi^*$  transition<sup>3</sup> in SubPc for clear visualization. **(b).1** DART analysis of C60 (analysed up to 13 nm thickness) deposited on the SubPc film in (a). **(b).2** Magnified view of the data of (b).1 around 2.1 eV for clear visualization. The optical response corresponding to the excitations into SubPc excitonic states is indicated by the label O1. All calculations were carried out for a differential change of  $\delta d = 1$  nm.

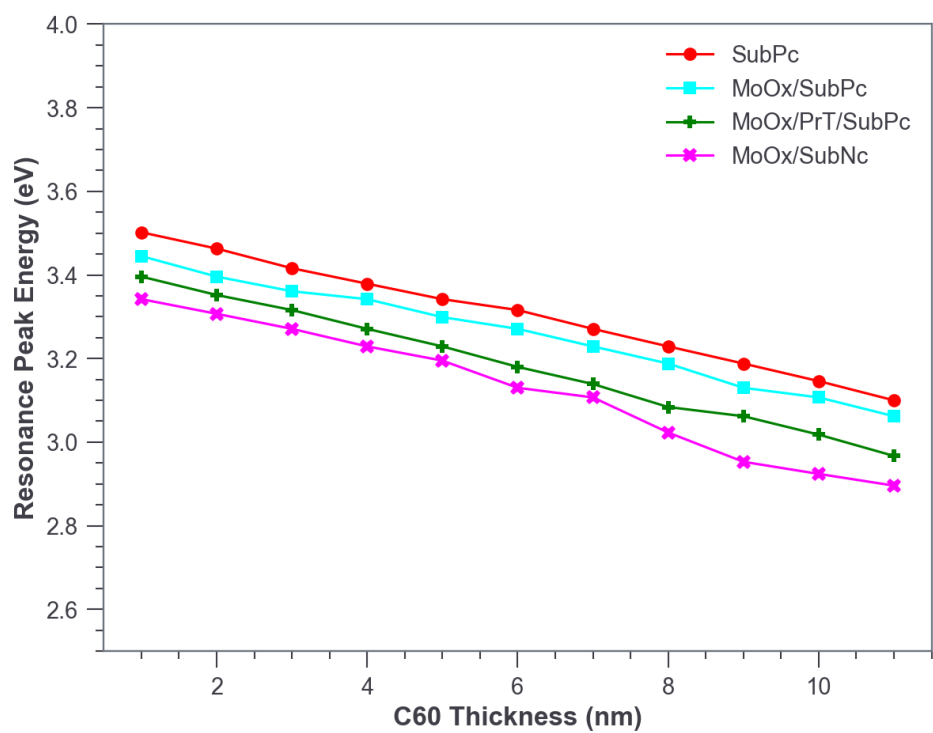

**Figure S11.** Energy values of the C60 resonance peaks as a function of C60 thickness obtained from the DART results in Figures 4, 6, S9 and S10.

## References

1. Fujiwara, H. *Spectroscopic ellipsometry : principles and applications*. (John Wiley, 2007).
2. Azzam, R. M. . & Bashara, N. . *Ellipsometry and polarized light*. (Amsterdam ; Oxford : North-Holland, 1977).
3. Morse, G. E. & Bender, T. P. Boron subphthalocyanines as organic electronic materials. *ACS Appl. Mater. Interfaces* **4**, 5055–5068 (2012).
4. Forker, R., Gruenewald, M. & Fritz, T. Optical differential reflectance spectroscopy on thin molecular films. *Annu. Reports Sect. 'C' (Physical Chem.* **108**, 34–68 (2012).
5. Gruenewald, M. *et al.* Impact of a molecular wetting layer on the structural and optical properties of tin(II)-phthalocyanine multilayers on Ag(111). *Phys. Rev. B* **93**, 115418 (2016).
6. Ye, H. *et al.* Efficiency enhancement of small molecule organic solar cells using hexapropyltruxene as an interface layer. *J. Mater. Chem. C* 26–29 (2020).
